# Supplementary material for: Generating Images with 3D Annotations Using Diffusion Models
Source: arXiv:2306.08103 source file (2024-04-03)
Supplement: Supplementary file 1 [file supp_more_images.tex]

\begin{figure}[t]
    \centering
    \begin{subfigure}[b]{}
    \centering
    \includegraphics[width=0.16\textwidth]{DST/1_0}
    \end{subfigure}
    \hfill
    \begin{subfigure}[b]{}
    \centering
    \includegraphics[width=0.16\textwidth]{DST/2_0}
    \end{subfigure}
    \hfill
    \begin{subfigure}[b]{}
    \centering
    \includegraphics[width=0.16\textwidth]{DST/3_0}
    \end{subfigure}
    \hfill
    \begin{subfigure}[b]{}
    \centering
    \includegraphics[width=0.16\textwidth]{DST/4_0}
    \end{subfigure}
    \hfill
    \begin{subfigure}[b]{}
    \centering
    \includegraphics[width=0.16\textwidth]{DST/5_0}
    \end{subfigure} \\
    \begin{subfigure}[b]{}
    \centering
    \includegraphics[width=0.16\textwidth]{DST/6_0}
    \end{subfigure}
    \hfill
    \begin{subfigure}[b]{}
    \centering
    \includegraphics[width=0.16\textwidth]{DST/7_0}
    \end{subfigure}
    \hfill
    \begin{subfigure}[b]{}
    \centering
    \includegraphics[width=0.16\textwidth]{DST/8_0}
    \end{subfigure}
    \hfill
    \begin{subfigure}[b]{}
    \centering
    \includegraphics[width=0.16\textwidth]{DST/9_1}
    \end{subfigure}
    \hfill
    \begin{subfigure}[b]{}
    \centering
    \includegraphics[width=0.16\textwidth]{DST/10_0}
    \end{subfigure} \\
    \begin{subfigure}[b]{}
    \centering
    \includegraphics[width=0.16\textwidth]{DST/11_0}
    \end{subfigure}
    \hfill
    \begin{subfigure}[b]{}
    \centering
    \includegraphics[width=0.16\textwidth]{DST/12_0}
    \end{subfigure}
    \hfill
    \begin{subfigure}[b]{}
    \centering
    \includegraphics[width=0.16\textwidth]{DST/13_0}
    \end{subfigure}
    \hfill
    \begin{subfigure}[b]{}
    \centering
    \includegraphics[width=0.16\textwidth]{DST/14_0}
    \end{subfigure}
    \hfill
    \begin{subfigure}[b]{}
    \centering
    \includegraphics[width=0.16\textwidth]{DST/15_0}
    \end{subfigure} \\
    \begin{subfigure}[b]{}
    \centering
    \includegraphics[width=0.16\textwidth]{DST/16_0}
    \end{subfigure}
    \hfill
    \begin{subfigure}[b]{}
    \centering
    \includegraphics[width=0.16\textwidth]{DST/17_0}
    \end{subfigure}
    \hfill
    \begin{subfigure}[b]{}
    \centering
    \includegraphics[width=0.16\textwidth]{DST/18_0}
    \end{subfigure}
    \hfill
    \begin{subfigure}[b]{}
    \centering
    \includegraphics[width=0.16\textwidth]{DST/19_0}
    \end{subfigure}
    \hfill
    \begin{subfigure}[b]{}
    \centering
    \includegraphics[width=0.16\textwidth]{DST/20_0}
    \end{subfigure} \\
    \begin{subfigure}[b]{}
    \centering
    \includegraphics[width=0.16\textwidth]{DST/21_0}
    \end{subfigure}
    \hfill
    \begin{subfigure}[b]{}
    \centering
    \includegraphics[width=0.16\textwidth]{DST/22_0}
    \end{subfigure}
    \hfill
    \begin{subfigure}[b]{}
    \centering
    \includegraphics[width=0.16\textwidth]{DST/23_0}
    \end{subfigure}
    \hfill
    \begin{subfigure}[b]{}
    \centering
    \includegraphics[width=0.16\textwidth]{DST/24_1}
    \end{subfigure}
    \hfill
    \begin{subfigure}[b]{}
    \centering
    \includegraphics[width=0.16\textwidth]{DST/25_0}
    \end{subfigure} \\
    \begin{subfigure}[b]{}
    \centering
    \includegraphics[width=0.16\textwidth]{DST/26_0}
    \end{subfigure}
    \hfill
    \begin{subfigure}[b]{}
    \centering
    \includegraphics[width=0.16\textwidth]{DST/27_0}
    \end{subfigure}
    \hfill
    \begin{subfigure}[b]{}
    \centering
    \includegraphics[width=0.16\textwidth]{DST/28_0}
    \end{subfigure}
    \hfill
    \begin{subfigure}[b]{}
    \centering
    \includegraphics[width=0.16\textwidth]{DST/29_0}
    \end{subfigure}
    \hfill
    \begin{subfigure}[b]{}
    \centering
    \includegraphics[width=0.16\textwidth]{DST/30_0}
    \end{subfigure} \\
    \begin{subfigure}[b]{}
    \centering
    \includegraphics[width=0.16\textwidth]{DST/31_0}
    \end{subfigure}
    \hfill
    \begin{subfigure}[b]{}
    \centering
    \includegraphics[width=0.16\textwidth]{DST/32_0}
    \end{subfigure}
    \hfill
    \begin{subfigure}[b]{}
    \centering
    \includegraphics[width=0.16\textwidth]{DST/33_0}
    \end{subfigure}
    \hfill
    \begin{subfigure}[b]{}
    \centering
    \includegraphics[width=0.16\textwidth]{DST/34_0}
    \end{subfigure}
    \hfill
    \begin{subfigure}[b]{}
    \centering
    \includegraphics[width=0.16\textwidth]{DST/35_0}
    \end{subfigure} \\
    \begin{subfigure}[b]{}
    \centering
    \includegraphics[width=0.16\textwidth]{DST/36_0}
    \end{subfigure}
    \hfill
    \begin{subfigure}[b]{}
    \centering
    \includegraphics[width=0.16\textwidth]{DST/37_0}
    \end{subfigure}
    \hfill
    \begin{subfigure}[b]{}
    \centering
    \includegraphics[width=0.16\textwidth]{DST/38_0}
    \end{subfigure}
    \hfill
    \begin{subfigure}[b]{}
    \centering
    \includegraphics[width=0.16\textwidth]{DST/39_0}
    \end{subfigure}
    \hfill
    \begin{subfigure}[b]{}
    \centering
    \includegraphics[width=0.16\textwidth]{DST/40_0}
    \end{subfigure} \\
    \begin{subfigure}[b]{}
    \centering
    \includegraphics[width=0.16\textwidth]{DST/41_0}
    \end{subfigure}
    \hfill
    \begin{subfigure}[b]{}
    \centering
    \includegraphics[width=0.16\textwidth]{DST/42_0}
    \end{subfigure}
    \hfill
    \begin{subfigure}[b]{}
    \centering
    \includegraphics[width=0.16\textwidth]{DST/43_0}
    \end{subfigure}
    \hfill
    \begin{subfigure}[b]{}
    \centering
    \includegraphics[width=0.16\textwidth]{DST/44_0}
    \end{subfigure}
    \hfill
    \begin{subfigure}[b]{}
    \centering
    \includegraphics[width=0.16\textwidth]{DST/45_0}
    \end{subfigure} \\
    \begin{subfigure}[b]{}
    \centering
    \includegraphics[width=0.16\textwidth]{DST/46_0}
    \end{subfigure}
    \hfill
    \begin{subfigure}[b]{}
    \centering
    \includegraphics[width=0.16\textwidth]{DST/47_0}
    \end{subfigure}
    \hfill
    \begin{subfigure}[b]{}
    \centering
    \includegraphics[width=0.16\textwidth]{DST/48_0}
    \end{subfigure}
    \hfill
    \begin{subfigure}[b]{}
    \centering
    \includegraphics[width=0.16\textwidth]{DST/49_0}
    \end{subfigure}
    \hfill
    \begin{subfigure}[b]{}
    \centering
    \includegraphics[width=0.16\textwidth]{DST/50_0}
    \end{subfigure}
    \caption{Samples images from our 3D-DST dataset.}
    \label{fig:sample_50}
\end{figure}
