# Supplementary material for: Generating Images with 3D Annotations Using Diffusion Models
Source: arXiv:2306.08103 source file (2024-04-03)
Supplement: Supplementary file 2 [file supp_class_iid_50.tex]

\begin{table}
\begin{center}
\begin{tabular}{ c|l } 
\hline
synset &class name \\
\hline
\underline{n01443537} &goldfish, Carassius auratus \\
n01514668 &cock \\
\underline{n01855672} &goose \\
\underline{n02007558} &flamingo \\
\underline{n02129165} &lion, king of beasts, Panthera leo \\
\underline{n02129604} &tiger, Panthera tigris \\
n02342885 &hamster \\
\underline{n02391049} &zebra \\
\underline{n02510455} &giant panda, panda, panda bear, coon bear, Ailuropoda melanoleuca \\
n02676566 &acoustic guitar \\
n02690373 &airliner \\
\underline{n02701002} &ambulance \\
n02747177 &ashcan, trash can, garbage can, wastebin, ash bin, ash-bin, ashbin, dustbin, trash barrel, trash bin \\
\underline{n02808440} &bathtub, bathing tub, bath, tub \\
n02814533 &beach wagon, station wagon, wagon, estate car, beach waggon, station waggon, waggon \\
\underline{n02843684} &birdhouse \\
n02930766 &cab, hack, taxi, taxicab \\
\underline{n02992529} &cellular telephone, cellular phone, cellphone, cell, mobile phone \\
n03063599 &coffee mug \\
n03085013 &computer keyboard, keypad \\
n03095699 &container ship, containership, container vessel \\
n03187595 &dial telephone, dial phone \\
n03201208 &dining table, board \\
\underline{n03452741} &grand piano, grand \\
n03642806 &laptop, laptop computer \\
n03658185 &letter opener, paper knife, paperknife \\
n03709823 &mailbag, postbag \\
\underline{n03710193} &mailbox, letter box \\
n03761084 &microwave, microwave oven \\
n03792782 &mountain bike, all-terrain bike, off-roader \\
n03891251 &park bench \\
n03938244 &pillow \\
n03977966 &police van, police wagon, paddy wagon, patrol wagon, wagon, black Maria \\
n03983396 &pop bottle, soda bottle \\
n03991062 &pot, flowerpot \\
n04004767 &printer \\
n04074963 &remote control, remote \\
\underline{n04146614} &school bus \\
n04263257 &soup bowl \\
n04330267 &stove \\
n04344873 &studio couch, day bed \\
n04380533 &table lamp \\
n04487081 &trolleybus, trolley coach, trackless trolley \\
\underline{n04552348} &warplane, military plane \\
n04554684 &washer, automatic washer, washing machine \\
n04557648 &water bottle \\
\underline{n07720875} &bell pepper \\
\underline{n07745940} &strawberry \\
\underline{n07753275} &pineapple, ananas \\
\underline{n07753592} &banana \\
\hline
\end{tabular}
\vspace{0.3cm}
\caption{The related ImageNet synsets and class names of the 50 classes used in 3D-DST classification. The 19 synsets with underlines are the classes overlapping with ImageNet-R that are used in OOD experiments.}
\vspace{-0.3cm}
\label{tab:supp_class_iid_50}
\end{center}
\end{table}
