# Supplementary material for: Generating Images with 3D Annotations Using Diffusion Models
Source: arXiv:2306.08103 source file (2024-04-03)
Supplement: Supplementary file 3 [file supp_LLM_simple_prompt.tex]

\begin{figure}[!t]
    \centering
    \begin{subfigure}[b]{}
    \centering
    \includegraphics[width=0.24\textwidth]{DST/5_0}
    \includegraphics[width=0.24\textwidth]{DST/9_1}
    \includegraphics[width=0.24\textwidth]{DST/14_0}
    \includegraphics[width=0.24\textwidth]{DST/15_0}
    \includegraphics[width=0.24\textwidth]{DST/23_0}
    \includegraphics[width=0.24\textwidth]{DST/24_1}
    \includegraphics[width=0.24\textwidth]{DST/48_0}
    \includegraphics[width=0.24\textwidth]{DST/50_0}
    \caption{3D-DST data with diverse prompts from LLM.}
    \end{subfigure}
    \hfill
    \begin{subfigure}[b]{}
    \centering
    \includegraphics[width=0.24\textwidth]{DST_simple/5_0}
    \includegraphics[width=0.24\textwidth]{DST_simple/9_0}
    \includegraphics[width=0.24\textwidth]{DST_simple/14_0}
    \includegraphics[width=0.24\textwidth]{DST_simple/15_0}
    \includegraphics[width=0.24\textwidth]{DST_simple/23_0}
    \includegraphics[width=0.24\textwidth]{DST_simple/24_0}
    \includegraphics[width=0.24\textwidth]{DST_simple/48_0}
    \includegraphics[width=0.24\textwidth]{DST_simple/50_0}
    \caption{3D-DST data with simple prompts.}
    \end{subfigure}
    \caption{Qualitative comparison between 3D-DST data generated with diverse prompts with LLM and simple prompts crafted by hand.}
    \label{fig:comparison}
\end{figure}
