# Supplementary material for: Generating Images with 3D Annotations Using Diffusion Models
Source: arXiv:2306.08103 source file (2024-04-03)
Supplement: Supplementary file 4 [file supp_ablation_datagen_pose.tex]

\begin{table}
\centering
{
\setlength{\tabcolsep}{1mm}{
\revision{
\begin{tabular}{llllllll}
    \toprule
    Methods & ACC@$\pi/6$ & ACC@$\pi/18$ & MedErr \\
    \midrule
    NeMo~\citep{Wang2021NeMo} & 70.6 {\scriptsize\textcolor{white}{$\uparrow$0.0}} & 46.5 {\scriptsize\textcolor{white}{$\uparrow$0.0}} & 23.6 {\scriptsize\textcolor{white}{$\uparrow$0.0}} \\
    \emph{\ \ w /} Rendering + BG2D & 75.9 {\scriptsize\textcolor{ablation_green}{($\uparrow$5.3)}} & 47.8 {\scriptsize\textcolor{ablation_green}{($\uparrow$1.3)}} & 17.1 {\scriptsize\textcolor{ablation_green}{($\downarrow$6.5)}} \\
    \emph{\ \ w /} Rendering + BG3D & 76.2 {\scriptsize\textcolor{ablation_green}{($\uparrow$5.6)}} & 49.3 {\scriptsize\textcolor{ablation_green}{($\uparrow$2.8)}} & 16.4 {\scriptsize\textcolor{ablation_green}{($\downarrow$7.2)}} \\
    \cellcolor{mygray-bg}{\emph{\ \ w /} 3D-DST (ours)} & \cellcolor{mygray-bg}{\textbf{79.2} {\scriptsize\textcolor{ablation_green}{($\uparrow$8.6)}}} & \cellcolor{mygray-bg}{\textbf{52.0} {\scriptsize\textcolor{ablation_green}{($\uparrow$5.5)}}} & \cellcolor{mygray-bg}{\textbf{14.1} {\scriptsize\textcolor{ablation_green}{($\downarrow$9.5)}}} \\
    \\[-14pt]
    \bottomrule
\end{tabular}}}}
\caption{\revision{\textbf{Ablation study of data generation methods on pose estimation.} We adopt the state-of-the-art 3D pose estimation model \citep{Wang2021NeMo} as the baseline model and compare the performance with different data generation methods. Please refer to Section~\ref{sec:supp_ablation_datagen} for specifics of each data generation approach.}}
\label{tab:exp-ablation-datagen-pose}
\end{table}
