# Supplementary material for: Generating Images with 3D Annotations Using Diffusion Models
Source: arXiv:2306.08103 source file (2024-04-03)
Supplement: Supplementary file 5 [file supp_dataset_size.tex]

\begin{table}[t]
\centering
{
\setlength{\tabcolsep}{1.5mm}{

\begin{tabular}{lcc}
    \toprule
    Methods & ResNet-50 & ViT-S  \\
    \midrule
    ImageNet-50 &   86.60 & 84.72 \\
    ImageNet-50 + \OursCls 1500 & 88.16 & 87.12  \\
    ImageNet-50 + \OursCls 2000 & 88.72 & 88.28 \\
    \cellcolor{mygray-bg}{ImageNet-50 + \OursCls 2500} & \cellcolor{mygray-bg}{\textbf{89.28}} & \cellcolor{mygray-bg}{\textbf{89.36}}  \\ 
    \bottomrule
\end{tabular}}}
\vspace{0.3cm}
\caption{Comparison of the effects of different dataset sizes when \OursCls contains 1500, 2000, and 2500 synthetic images per class, respectively. We evaluate Top-1 accuracy of image classification on ImageNet-50 for ResNet-50 and ViT-S. Experiments show that only using \OursCls with 1500 per class can already improve the accuracy a lot, and using more data can further improve the classification performance of all the models.}
\vspace{-0.3cm}
\label{tab:supp-dataset-size}
\end{table}
