# Supplementary material for: Generating Images with 3D Annotations Using Diffusion Models
Source: arXiv:2306.08103 source file (2024-04-03)
Supplement: Supplementary file 6 [file supp_simple.tex]

\begin{table}[t]
\centering
{
\setlength{\tabcolsep}{1.5mm}{

\begin{tabular}{lcc}
    \toprule
    Methods & ResNet-50 & ViT-S \\
    \midrule
    ImageNet-50 &   86.60 & 84.72 \\
    ImageNet-50 + 3D-DST wo LLM prompts & 88.96 & 88.72 \\
     & {\small \textcolor{ablation_green}{($\uparrow$2.36)}}&  {\small \textcolor{ablation_green}{($\uparrow$4.00)}}\\
    \cellcolor{mygray-bg}{ImageNet-50 + \OursCls (ours)} & \cellcolor{mygray-bg}{\textbf{89.28}} & \cellcolor{mygray-bg}{\textbf{89.36}}  \\\cellcolor{mygray-bg}{}
    & \cellcolor{mygray-bg}{{\small \textcolor{ablation_green}{($\uparrow$2.68)}}} & \cellcolor{mygray-bg}{{\small \textcolor{ablation_green}{($\uparrow$4.64)}}} \\
    \\[-14pt]
    \bottomrule
\end{tabular}}}
\vspace{0.3cm}
\caption{Top-1 accuracy of image classification on ImageNet-50. We evaluate representative models, ResNet-50 and ViT-S. We compare the performances when models are (1) trained purely on ImageNet-50, (2) pretrained on 3D-DST data generated without using LLM prompts (only use simple prompts like class names and keywords from the CAD model descriptions), and then finetuned on ImageNet, (3) pretrained on 3D-DST data, and finetuned on ImageNet-50. Experiments show that our 3D-DST data can help boost the classification accuracy of all the models by a large margin, and using LLM prompts can help achieve better results.}
\vspace{-0.3cm}
\label{tab:supp-simple}
\end{table}
